# Supplementary material for: Toward a Data Processing Pipeline for Mobile-Phone Tracking Data
Source: arXiv:2507.00952 ancillary file (2025-07-01)
Supplement: Supplementary file 1 [file supplement.pdf]

# Supplementary material for "Toward a Data Processing Pipeline for Mobile-Phone Tracking Data"

Marcin Jurek<sup>\*1</sup>, Catherine A. Calder<sup>2</sup>, Corwin Zigler<sup>3</sup>, Bethany Boettner<sup>4</sup>,  
and Christopher R. Browning<sup>5</sup>

<sup>1</sup>Department of Statistics and Data Science, Southern Methodist University

<sup>2</sup>Department of Statistics and Data Sciences, University of Texas at Austin

<sup>3</sup>Department of Biostatistics, Brown University

<sup>4</sup>Institute for Population Research, Ohio State University

<sup>5</sup>Department of Sociology, Ohio State University

July 1, 2025

## **S1 Sample trajectory and imputations used in numerical simulations**

---

<sup>\*</sup>marcinjurek1988@gmail.com

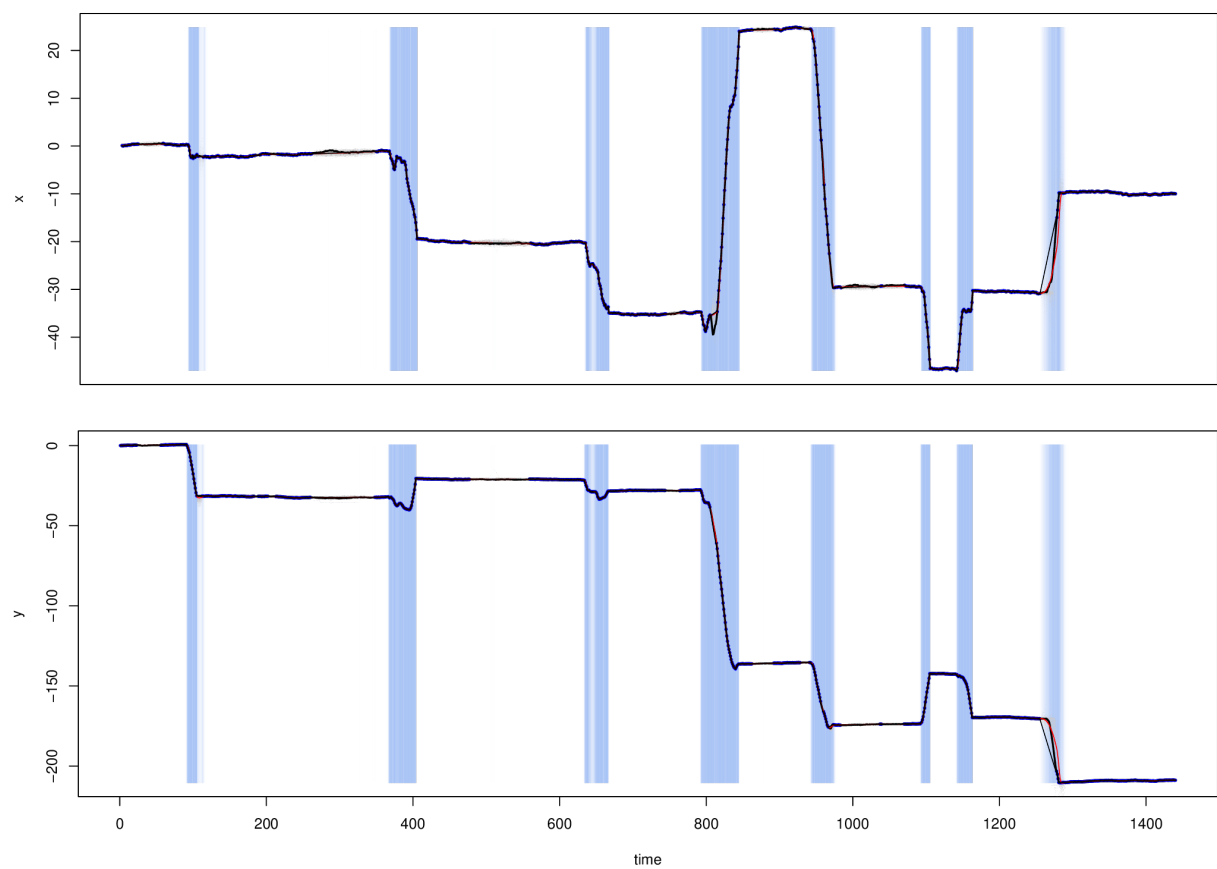

Figure S1: One of the simulated trajectories and segmentation results produced by the statistical algorithm

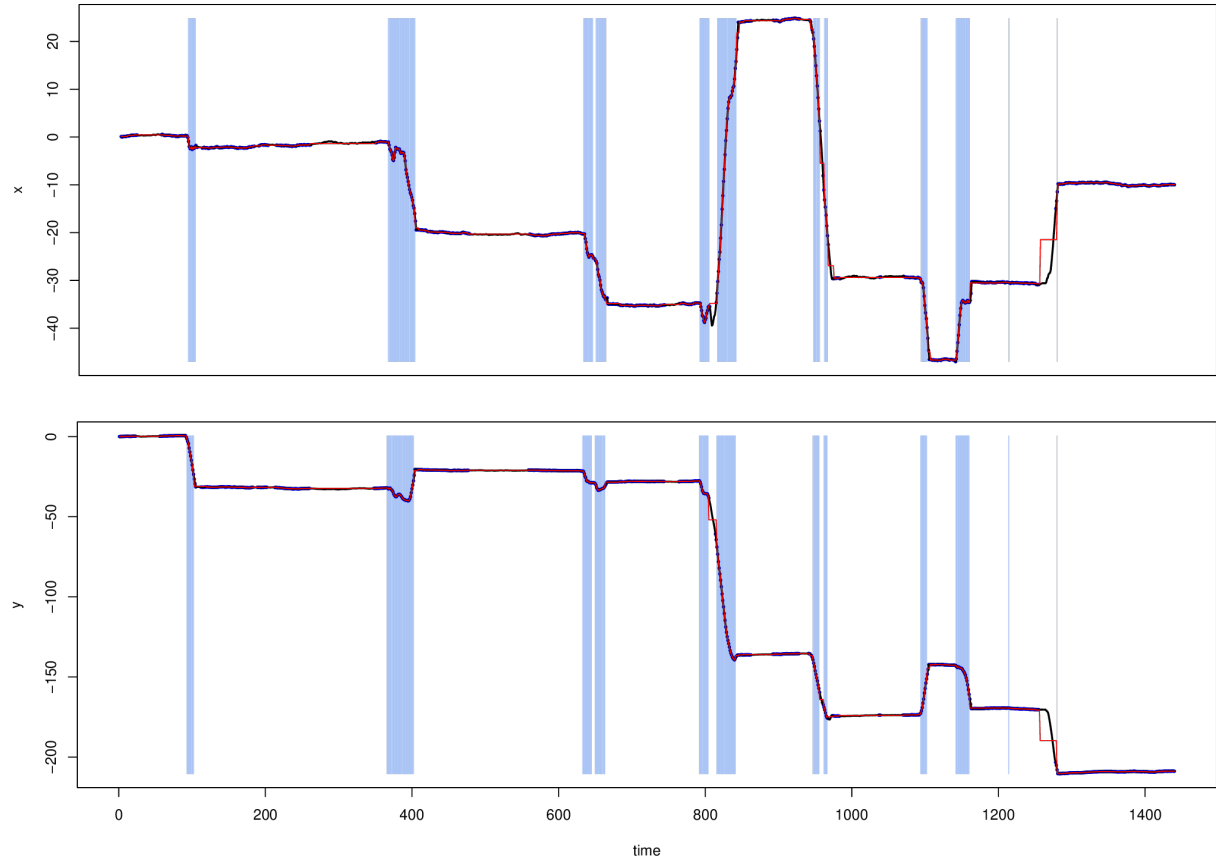

Figure S2: One of the simulated trajectories and segmentation results produced by the binning algorithm

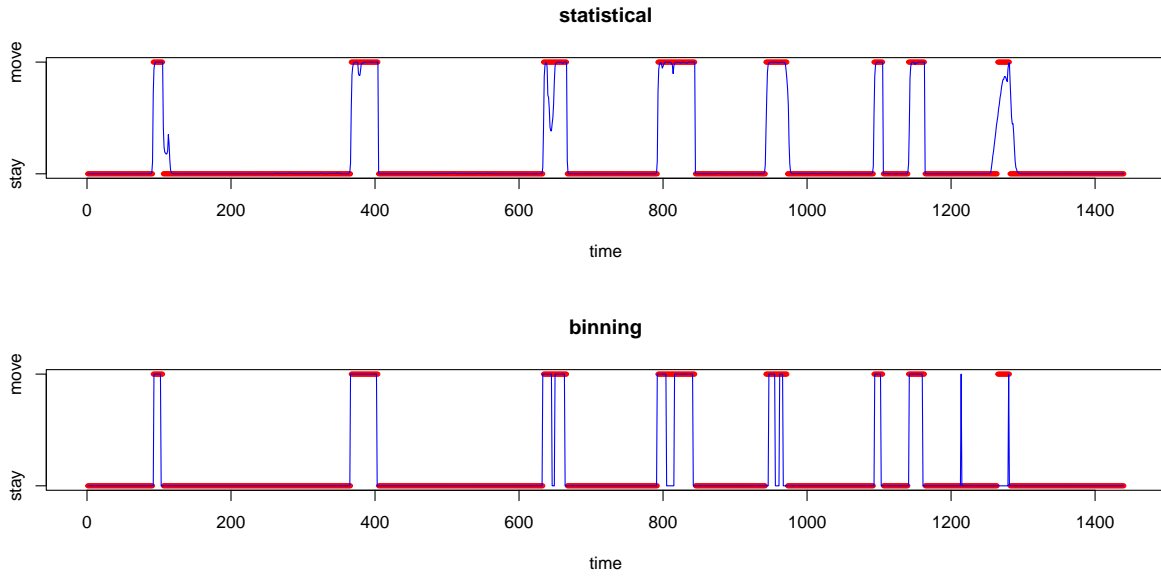

Figure S3: Segmentation produced by either method. Red line stands for the true segmentation (which is known in this case - unlike in the case of real data - because the trajectory was simulated).

## S2 Additional plots for AHDC data.

### S2.1 Results for data set 2

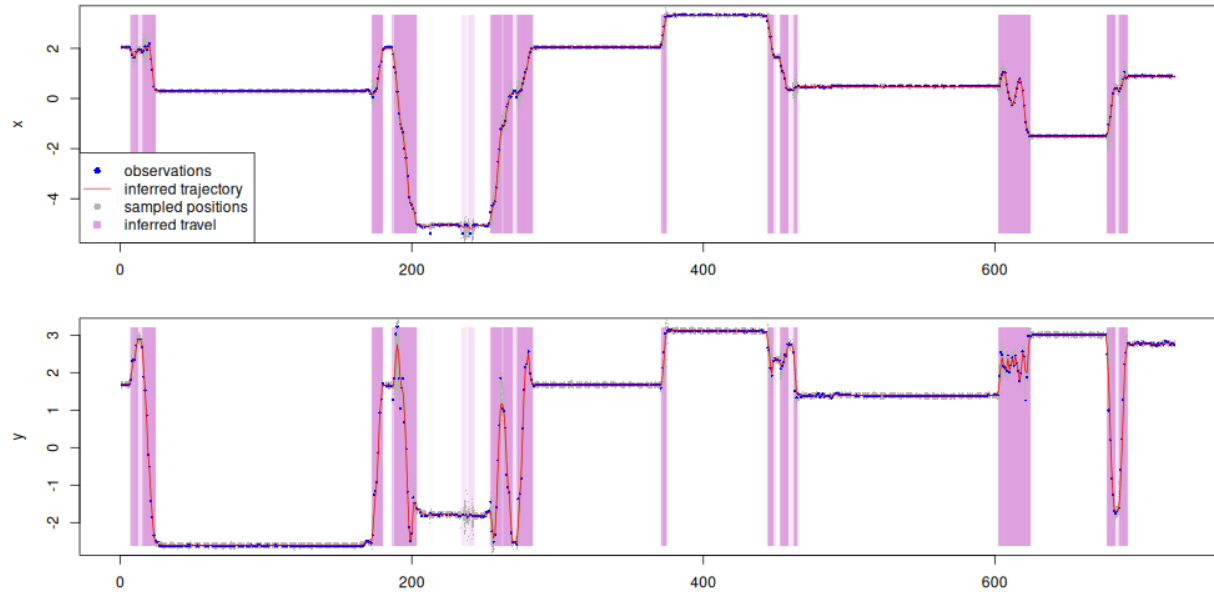

Figure S4: The top panel corresponds to the  $x$  coordinate over time, the bottom panels shows the  $y$  coordinate as a function of time. The intensity of the purple background indicates the estimated probability of the individual being in motion at a given time point (more intense color means higher probability). The grey dots represent samples from the approximate smoothing distribution and indicate uncertainty. The red line is the point estimate of the individual's location and blue dots are observations.

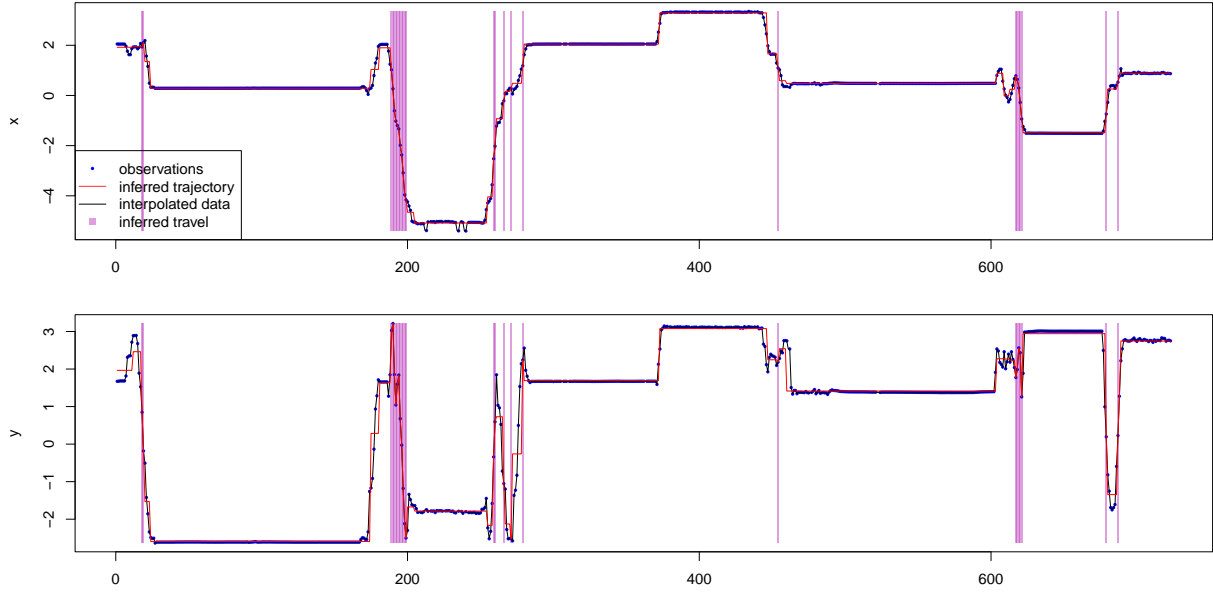

Figure S5: The results of processing the data using the binning algorithm. The blue dots represent observations and interpolation, whenever the true data is missing. The red line corresponds to the trajectory generated by the algorithm. Travel periods are indicated in light blue.

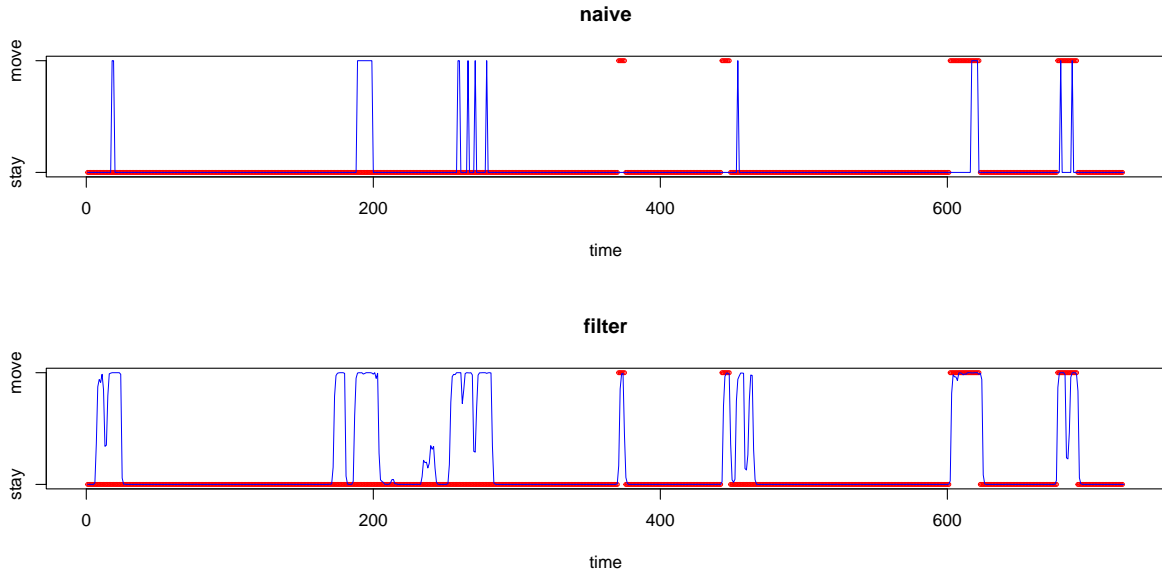

Figure S6: Comparison of various segmentation methods. The top panel shows the  $x$  coordinate as a function of time. The second panel shows the segmentation produces by Algorithm 1The “binning algorithm”`algocf.1`. The third one shows the probability of the individual being in motion as a function of time obtained using the statistical algorithm proposed in this paper. The last panel displays the segmentation provided by the participant. Note that the plot shows only the data for  $t \in [400, 1300]$ .

## S2.2 Results for data set 3

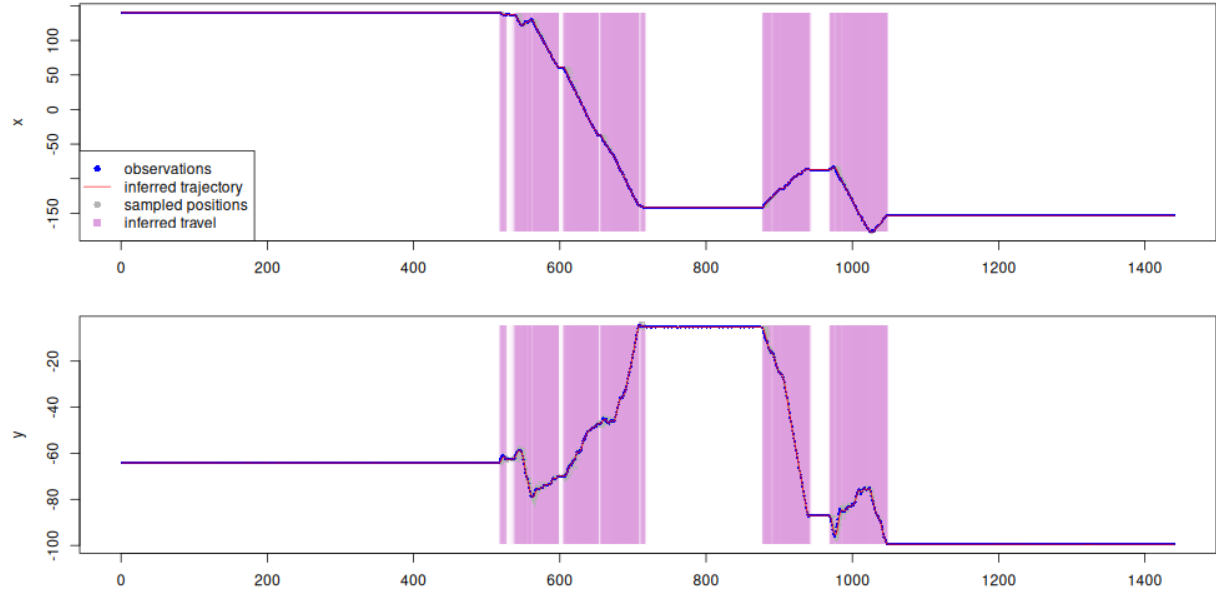

Figure S7: The top panel corresponds to the  $x$  coordinate over time, the bottom panels shows the  $y$  coordinate as a function of time. The intensity of the purple background indicates the estimated probability of the individual being in motion at a given time point (more intense color means higher probability). The grey dots represent samples from the approximate smoothing distribution and indicate uncertainty. The red line is the point estimate of the individual's location and blue dots are observations.

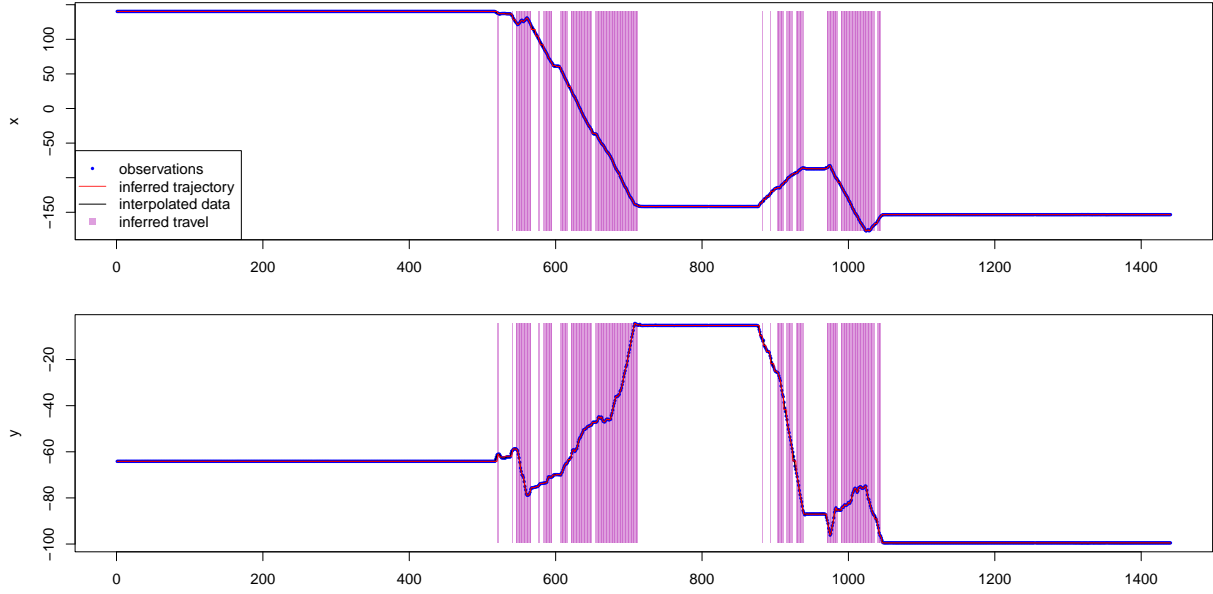

Figure S8: The results of processing the data using the binning algorithm. The blue dots represent observations and interpolation, whenever the true data is missing. The red line corresponds to the trajectory generated by the algorithm. Travel periods are indicated in light blue.

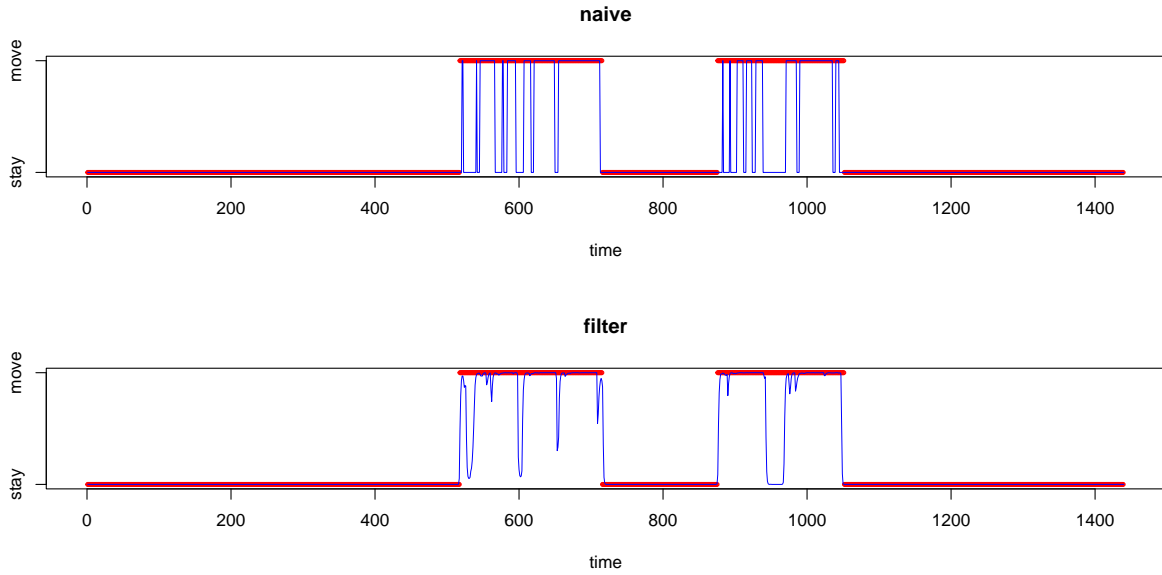

Figure S9: Comparison of various segmentation methods. The top panel shows the  $x$  coordinate as a function of time. The second panel shows the segmentation produces by Algorithm 1The “binning algorithm”`algotcf.1`. The third one shows the probability of the individual being in motion as a function of time obtained using the statistical algorithm proposed in this paper. The red line shows the segmentation provided by the participant - note that this is not necessarily ground truth. Note that the plot shows only the data for  $t \in [400, 1300]$ .
